# Supplementary material for: Explaining Relationships Between Scientific Documents
Source: arXiv:2002.00317 source file (2021-08-12)
Supplement: Supplementary file 1 [file appendix2.tex]

\xinyi{Added to appendix some analysis I am unsure about whether/where to put.}
\section{Analysis of Token-Wise Overlap}
\begin{table*}
\centering
\begin{tabular}{lcccc}
\hline
& \fieldheading{None} & \fieldheading{Cited abs} & \fieldheading{Cited tfidf} & \fieldheading{Cited entities}\\
\hline
None & N/A & 18.60 & 22.05 & 22.22\\
Principal abs x & 22.62 & 32.52 & 35.65 & 35.75\\
Principal intro x & 33.15 & 41.56 & 43.66 & 43.74\\
\hline
\end{tabular}
\caption{\label{table:overlap} Token-wise overlap with gold citation sentence.}
\end{table*}

\section{Oracle Study}
\begin{figure}[H]
    \centering
    \includegraphics[width=0.4\textwidth]{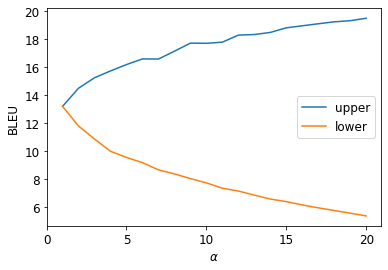}
    \caption{Upper and lower bounds of BLEU for different choices of $k$.}
    \label{fig:bounds}
\end{figure}

\section{Auto-Completion}
Given the first three words of the citation sentence, the BLEU score of the rest is 21.38.

\begin{table*}[t]
    \centering
    \begin{tabular}{rlrrrrr}
        \toprule
         && {\bf BLEU} & {\bf ACL-BLEU} & {\bf Rouge-1} & {\bf Rouge-2} & {\bf Rouge-L} \\ \toprule
        \multirow{6}{*}{Sentence\textsc{SciGen}} & \source~abs $\times$ cited abs &9.82 &10.40 & 10.7 & 0.6 & 8.4   \\
        &\source~abs $\times$ cited intro &9.39 & 9.82 &    10.7 &  0.6 &  8.4 \\
        &\source~abs $\times$ cited sample &9.60 &10.48 &   10.7 &  0.7  &  8.5 \\ \cline{2-7}
        &\source~intro $\times$ cited abs &9.92 &11.22 &    11.1 &  1.0 &  8.7 \\
        &\source~intro $\times$ cited intro &9.80 &10.54 &   1.1  &   1.1 &   8.8  \\
        &\source~intro $\times$ cited sample & 9.81 & 10.31 &    10.9  &  0.9 &  8.7 \\
        \midrule \midrule
        %\cline{2-7}
        \multirow{3}{*}{IR} & \source~abs $\times$ cited abs& 9.93 & 10.50  &   14.2 &  0.7  &  9.7 \\
        & \hspace{1em} + MERT (BLEU)& 10.23 & 10.29  &  14.3 &  0.7  &  9.8 \\
        & no \source~$\times$ cited abs & 9.79 &-  &   14.1  &  0.6  &  9.6 \\
        
        \bottomrule
    \end{tabular}
    \caption{Automatic evaluation of generated texts of our IR and sentence-based {\sc SciGen} models. The ACL-BLEU column denotes the BLEU scores of the subset of examples we use for human evaluation. \label{tab:auto}}
\end{table*}

\begin{table*}[ht]
    \centering
    \small
    \begin{tabularx}{\textwidth}{X}
    \toprule 
        %  {\bf Source} \\
        %  Learning to classify unseen class samples at test time is popularly referred to as zero-shot learning (ZSL). If test samples can be from training (seen) as well as unseen classes, it is a more challenging problem \ldots \\
        %  \vspace{-0.3em}
        %  {\bf Cited} \\
        %  State-of-the-art methods for zero-shot visual recognition formulate learning as a joint embedding problem of images and side information. In these formulations the current best complement to visual features are attributes \ldots \\
        %           \vspace{-0.3em}
        %  {\bf GPT} \\
        %   Nevertheless, our model is able to obtain competitive results with ({\it Cited}). \\ \vspace{-0.3em}
        %  {\bf IR} \\
        %   ({\it Cited}). \\ \vspace{-0.3em}
        %  {\bf Citing sentence} \\
        %   For CUB dataset, we use CNN-RNN textual features  ({\it Cited}) as class attributes, similar to the approaches mentioned in Table 5 and 2. \\ \hline  \hline 
                   {\bf Source} \\
       Secure communication over a wiretap channel is considered in the disadvantaged wireless environment, where the eavesdropper channel is (possibly much) better than the main channel. \ldots \\\vspace{-0.3em}
         {\bf Cited} \\
        We consider the secure transmission of information over an ergodic fading channel in the presence of an eavesdropper. Our eavesdropper can be viewed as th     e wireless counterpart of Wyner's wiretapper. \ldots \\\vspace{-0.3em}
         {\bf Sentence-based SciGen} \\
         In  ({\it Cited}), an optimal SWIPT scheme was proposed with perfect CSIT. \\\vspace{-0.3em}
         {\bf IR} \\
        Consider the channel model shown in Figure 1 , which reflects the understanding that in an adversarial game in modern communication systems, it is the interference effects on wideband receiver front-ends rather than the baseband processing that is the significant detriment  ({\it Cited}).\\\vspace{-0.3em}
         {\bf Citing sentence} \\
          However, public discussion schemes result in low secrecy rates in scenarios of interest (as discussed in detail in ({\it Cited})), and the technique proposed here can be used in conjunction with public discussion approaches when two-way communication is possible. \\
          \hline \hline
            {\bf Source} \\ Indian epics have not been analyzed computationally to the extent that Greek epics have. In this paper, we show how interesting in     sights can be derived from the ancient epic Mahabharata by applying a variety of analytical techniques based on a combination of natural language processing, sentiment/emotion analysis and social network analysis methods.
            \ldots \\\vspace{-0.3em}
         {\bf Cited} \\
        We present a method for extracting social networks from literature, namely, nineteenth-century British novels and serials. We derive the networks from dialogue interactions, and thus our method depends on the ability to determine when two characters are in conversation. \ldots \\\vspace{-0.3em}
         {\bf Sentence-based SciGen} \\
        The authors of ({\it Cited}) presented a method of characterizing the motivations for writing the essays by examining the topical influence of characters\\\vspace{-0.3em}
         {\bf IR} \\
        We present an approach to the extraction of family relations from literary narrative, which incorporates a technique for utterance attribution proposed recently by ({\it Cited}) .\\\vspace{-0.3em}
         {\bf Citing sentence} \\
          Robert ({\it Cited}) defined the eight basic emotion types. \\
          \hline \hline
           {\bf Source} \\ Automatic description generation from natural images is a challenging problem that has recently received a large amount of interest from the computer vision and natural language processing communities. In this survey,
            \ldots \\\vspace{-0.3em}
         {\bf Cited} \\
        Crowd-sourcing approaches such as Amazon's Mechanical Turk (MTurk) make it possible to annotate or collect large amounts of linguistic data at a relatively low cost and high speed. However, MTurk offers only limited control over who is allowed to particpate in a particular task. \ldots \\\vspace{-0.3em}
        {\bf Sentence-based SciGen} \\
        Evaluation was performed using the CIDEr metric ({\it Cited}).\\\vspace{-0.3em}
         {\bf IR} \\
       The last and the most challenging dataset, Pascal1k ({\it Cited}), is a collection of images with associated natural language sentences.\\\vspace{-0.3em}
         {\bf Citing sentence} \\
          The Pascal1K sentence dataset ({\it Cited}) is a dataset which is commonly used as a benchmark for evaluating the quality of description generation systems. \\
          \bottomrule
    \end{tabularx}
    \caption{Randomly selected examples of system inputs and outputs from validation set.}
    \label{tab:examples}
\end{table*}
}

\begin{table*}[ht]
    \centering
    \small
    \begin{tabularx}{\textwidth}{X}
    \toprule 
        %  {\bf Source} \\
        %  Learning to classify unseen class samples at test time is popularly referred to as zero-shot learning (ZSL). If test samples can be from training (seen) as well as unseen classes, it is a more challenging problem \ldots \\
        %  \vspace{-0.3em}
        %  {\bf Cited} \\
        %  State-of-the-art methods for zero-shot visual recognition formulate learning as a joint embedding problem of images and side information. In these formulations the current best complement to visual features are attributes \ldots \\
        %           \vspace{-0.3em}
        %  {\bf GPT} \\
        %   Nevertheless, our model is able to obtain competitive results with ({\it Cited}). \\ \vspace{-0.3em}
        %  {\bf IR} \\
        %   ({\it Cited}). \\ \vspace{-0.3em}
        %  {\bf Citing sentence} \\
        %   For CUB dataset, we use CNN-RNN textual features  ({\it Cited}) as class attributes, similar to the approaches mentioned in Table 5 and 2. \\ \hline  \hline 
                   {\bf \source} \\
       Secure communication over a wiretap channel is considered in the disadvantaged wireless environment, where the eavesdropper channel is (possibly much) better than the main channel. \ldots \\\vspace{-0.3em}
         {\bf Cited} \\
        We consider the secure transmission of information over an ergodic fading channel in the presence of an eavesdropper. Our eavesdropper can be viewed as th     e wireless counterpart of Wyner's wiretapper. \ldots
        \\\vspace{-0.3em}
         {\bf IE representation Input}
         \xinyi{newly added}\\
         perfect information-theoretic secrecy
         \ent full csi assumption \ent legitimate channel csi \ent low-complexity on/off power transmission scheme \ldots \tfidf e,(j+1 \tfidf wiretapper \tfidf gains \ldots
         \\\vspace{-0.3em}
         {\bf Sentence-Based SciGen Output} \\
         In  ({\it Cited}), an optimal SWIPT scheme was proposed with perfect CSIT. \\\vspace{-0.3em}
         {\bf IR} \\
        Consider the channel model shown in Figure 1 , which reflects the understanding that in an adversarial game in modern communication systems, it is the interference effects on wideband receiver front-ends rather than the baseband processing that is the significant detriment  ({\it Cited}).\\\vspace{-0.3em}
         {\bf Citing sentence} \\
          However, public discussion schemes result in low secrecy rates in scenarios of interest (as discussed in detail in ({\it Cited})), and the technique proposed here can be used in conjunction with public discussion approaches when two-way communication is possible. \\
          \hline \hline
            {\bf \source} \\ Indian epics have not been analyzed computationally to the extent that Greek epics have. In this paper, we show how interesting in     sights can be derived from the ancient epic Mahabharata by applying a variety of analytical techniques based on a combination of natural language processing, sentiment/emotion analysis and social network analysis methods.
            \ldots \\\vspace{-0.3em}
         {\bf Cited} \\
        We present a method for extracting social networks from literature, namely, nineteenth-century British novels and serials. We derive the networks from dialogue interactions, and thus our method depends on the ability to determine when two characters are in conversation. \ldots
        \\\vspace{-0.3em}
        {\bf IE representation Input} \\
        features \ent approach \ent talkative social networks \ent nineteenth-century european fiction \ent baseline social networks \ent conversation connections \ldots \tfidf bakhtin \tfidf british \tfidf correlation \ldots
        \\\vspace{-0.3em}
         {\bf Sentence-Based SciGen Output} \\
        The authors of ({\it Cited}) presented a method of characterizing the motivations for writing the essays by examining the topical influence of characters\\\vspace{-0.3em}
         {\bf IR} \\
        We present an approach to the extraction of family relations from literary narrative, which incorporates a technique for utterance attribution proposed recently by ({\it Cited}) .\\\vspace{-0.3em}
         {\bf Citing sentence} \\
          Robert ({\it Cited}) defined the eight basic emotion types. \\
          \hline \hline
           {\bf \source} \\ Automatic description generation from natural images is a challenging problem that has recently received a large amount of interest from the computer vision and natural language processing communities. In this survey,
            \ldots \\\vspace{-0.3em}
         {\bf Cited} \\
        Crowd-sourcing approaches such as Amazon's Mechanical Turk (MTurk) make it possible to annotate or collect large amounts of linguistic data at a relatively low cost and high speed. However, MTurk offers only limited control over who is allowed to particpate in a particular task. \ldots
        \\\vspace{-0.3em}
        {\bf IE representation Input}\\
        quality control test \ent online translation system \ent linguistic data collection \ent turker \ent amazon 's mechanical turk -lrb- mturk -rrb- \ent tasks \tfidf pascal \tfidf misspellings \tfidf grammar \ldots
        \\\vspace{-0.3em}
        {\bf Sentence-Based SciGen Output} \\
        Evaluation was performed using the CIDEr metric ({\it Cited}).\\\vspace{-0.3em}
         {\bf IR} \\
       The last and the most challenging dataset, Pascal1k ({\it Cited}), is a collection of images with associated natural language sentences.\\\vspace{-0.3em}
         {\bf Citing sentence} \\
          The Pascal1K sentence dataset ({\it Cited}) is a dataset which is commonly used as a benchmark for evaluating the quality of description generation systems. \\
          \bottomrule
    \end{tabularx}
    \caption{Randomly selected examples of system inputs and outputs from validation set. \kelvin{Add an appendix and shove this there?}}
    \label{tab:examples}
\end{table*}
